# Supplementary material for: Hyperbolic Multimodal Representation Learning for Biological Taxonomies
Source: arXiv:2508.16744 source file (2025-08-22)
Supplement: Supplementary file 1 [file supplement.tex]

% ICCV 2025 Paper Template

\documentclass[10pt,twocolumn,letterpaper]{article}

%%%%%%%%% PAPER TYPE  - PLEASE UPDATE FOR FINAL VERSION
% \usepackage{iccv}              % To produce the CAMERA-READY version
\usepackage[review]{iccv}      % To produce the REVIEW version
% \usepackage[pagenumbers]{iccv} % To force page numbers, e.g. for an arXiv version

% Import additional packages in the preamble file, before hyperref
\input{preamble}

% It is strongly recommended to use hyperref, especially for the review version.
% hyperref with option pagebackref eases the reviewers' job.
% Please disable hyperref *only* if you encounter grave issues, 
% e.g. with the file validation for the camera-ready version.
%
% If you comment hyperref and then uncomment it, you should delete *.aux before re-running LaTeX.
% (Or just hit 'q' on the first LaTeX run, let it finish, and you should be clear).
\definecolor{iccvblue}{rgb}{0.21,0.49,0.74}
\usepackage[pagebackref,breaklinks,colorlinks,allcolors=iccvblue]{hyperref}

%%%%%%%%% PAPER ID  - PLEASE UPDATE
 % *** Enter the Paper ID here

%%%%%%%%% TITLE - PLEASE UPDATE
\title{Hyperbolic Multimodal Representation Learning for Biological Taxonomy}

%%%%%%%%% AUTHORS - PLEASE UPDATE
\author{First Author\\
Institution1\\
Institution1 address\\
{\tt\small firstauthor@i1.org}
% For a paper whose authors are all at the same institution,
% omit the following lines up until the closing ``}''.
% Additional authors and addresses can be added with ``\and'',
% just like the second author.
% To save space, use either the email address or home page, not both
\and
Second Author\\
Institution2\\
First line of institution2 address\\
{\tt\small secondauthor@i2.org}
}

\begin{document}
\maketitle

\input{sec/6_appendix_tables_all}

% {
%     \small
%     \bibliographystyle{ieeenat_fullname}
%     \bibliography{main}
% }

\end{document}
